# Supplementary material for: Seer: Predictive Runtime Kernel Selection for Irregular Problems
Source: arXiv:2403.17017 source file (2024-02-19)
Supplement: Supplementary file 1 [file appendix.tex]

% LaTeX template for Artifact Evaluation V20201122
%
% Prepared by 
% * Grigori Fursin (cTuning foundation, France) 2014-2020
% * Bruce Childers (University of Pittsburgh, USA) 2014
%
% See examples of this Artifact Appendix in
%  * SC'17 paper: https://dl.acm.org/citation.cfm?id=3126948
%  * CGO'17 paper: https://www.cl.cam.ac.uk/~sa614/papers/Software-Prefetching-CGO2017.pdf
%  * ACM ReQuEST-ASPLOS'18 paper: https://dl.acm.org/citation.cfm?doid=3229762.3229763
%
% (C)opyright 2014-2020
%
% CC BY 4.0 license
%

\clearpage 
\appendix
\section{Artifact Appendix}

%%%%%%%%%%%%%%%%%%%%%%%%%%%%%%%%%%%%%%%%%%%%%%%%%%%%%%%%%%%%%%%%%%%%%
\subsection{Abstract}

Our framework, \emph{Seer}, addresses a complex problem of mapping sparse-irregular problems to the respective highest-performing kernel implementations, we present our work as a generalized abstraction extensible to other kernels and algorithms using a simple API. To showcase our framework, we conduct a case study in Sparse Matrix Vector Multiplication (SpMV), in which Seer predicts the best strategy for a given dataset with an improvement of 2 times over the best single iteration kernel across the entire SuiteSparse Matrix Collection dataset.

\subsection{Artifact check-list (meta-information)}

More detailed information available within the artifact's README file.

\begin{itemize}
  \item {\bf Data set: } Included, small CSV files with runtime information for Seer to process.
  \item {\bf Run-time environment: } Ubuntu 20/22.04, Dockerfile provided that installs all requirements (python packages).
  \item {\bf Hardware: } No specific hardware needed.
  \item {\bf Metrics: } Execution time is being compared within the plots. We evaluate our execution time against the fastest (``oracle'') kernel for all matrices.
  \item {\bf Output: } 10 plots generated after the scripts finish, see Section~\ref{sec:expected} for a list of expected plots.
  \item {\bf Experiments: } README explains the experimental setup, and provides a way to setup experiments using a Dockerfile or manually. 
  \item {\bf How much disk space required (approximately)?: } 100 MB
  \item {\bf How much time is needed to prepare workflow (approximately)?: } 4 mins using the docker setup, considerably faster if latest Ubuntu image is cached within docker.
  \item {\bf How much time is needed to complete experiments (approximately)?: } Less than 1 min with provided python scripts.
  \item {\bf Publicly available?: } No.
\end{itemize}

%%%%%%%%%%%%%%%%%%%%%%%%%%%%%%%%%%%%%%%%%%%%%%%%%%%%%%%%%%%%%%%%%%%%%
\subsection{Description}

\subsubsection{How to access}

Only available as a *.zip file uploaded to the CGO 2024 Artifact Evaluation website. The tool will separately be made available for public use in the future. For the evaluation purposes, we are not seeking the ``Artifact Available'' badge.

%%%%%%%%%%%%%%%%%%%%%%%%%%%%%%%%%%%%%%%%%%%%%%%%%%%%%%%%%%%%%%%%%%%%%
\subsection{Installation}

To start out, it's easiest to get set up using docker. The included docker file \lstinline{docker/Dockerfile} sets up the operating system and all the required dependencies. But to use docker, we need to install it first. A guide for installing docker can be found here: \url{https://docs.docker.com/engine/install/ubuntu/}. We have included a docker setup for \emph{Seer} which will install the requirements to run Seer.

{\small
\begin{lstlisting}
  cd <project-root>
  ./docker/build
  ./docker/run
\end{lstlisting}
}

%%%%%%%%%%%%%%%%%%%%%%%%%%%%%%%%%%%%%%%%%%%%%%%%%%%%%%%%%%%%%%%%%%%%%
\subsection{Experiment workflow}

For this setup, we've set the environment up to replicate the paper's results as closely as possible. From here, we can run the following two commands in our docker container to generate the models and create plots of the models performance on single and multi-iteration workloads.

{\small
\begin{lstlisting}
  python3 single_iteration.py
  python3 multi_iteration.py
\end{lstlisting}
}

%%%%%%%%%%%%%%%%%%%%%%%%%%%%%%%%%%%%%%%%%%%%%%%%%%%%%%%%%%%%%%%%%%%%%
\subsection{Evaluation and expected results}
\label{sec:expected}

To view and evaluate the generated plots, navigate to ./seer/plots/ directory and use a browser or viewer of your choice to open the .svg files. These should match approximately to the ones included in the paper. The expected outputs of the plot generation, and their corresponding figures in the paper are:

{\small
\begin{itemize}
  \item Figure 5a: seer/plots/single\_iteration/nlpkkt200.svg
  \item Figure 5b: seer/plots/single\_iteration/matrix-new\_3.svg
  \item Figure 5c: seer/plots/single\_iteration/Ga41As41H72.svg
  \item Figure 5d: seer/plots/single\_iteration/aggregate.svg
  \item Figure 7a: seer/plots/multi\_iteration/CurlCurl\_3\_1iter.svg
  \item Figure 7b: seer/plots/multi\_iteration/CurlCurl\_3\_19iter.svg
  \item Figure 7c: seer/plots/multi\_iteration/G3\_Circuit\_1iter.svg
  \item Figure 7d: seer/plots/multi\_iteration/G3\_Circuit\_19iter.svg
  \item Figure 7e: seer/plots/multi\_iteration/pwtk\_1iter.svg
  \item Figure 7f: seer/plots/multi\_iteration/pwtd\_19iter.svg
\end{itemize}
}
%%%%%%%%%%%%%%%%%%%%%%%%%%%%%%%%%%%%%%%%%%%%%%%%%%%%%%%%%%%%%%%%%%%%%
\subsection{Experiment customization}

We've included dataset in the Seer directory (seer/data/) as simple CSV (comma-separated values), which we can use to validate the Seer concept presented in the paper. This data can also be replaced with any of user's own kernel runtimes or metrics. Brief description of provided data:

{\small
\begin{itemize}
  \item \textbf{elapsed.csv}: The elapsed time of individual kernels on the SuiteSparse Matrix Collection dataset,
  \item \textbf{metadata.csv}: The metadata collection time on the data set, and
  \item \textbf{preprocess.csv}: The amount of preprocessing involved in each kernel.
\end{itemize}
}
